# Supplementary material for: Scrambling Ability of Quantum Neural Networks Architectures
Source: arXiv:2011.07698 source file (2020-11-16)
Supplement: Supplementary file 1 [file sm_QS.pdf]

# Supplemental Material for " Scrambling Ability of Quantum Neural Networks Architectures"

Yadong Wu,[1] Pengfei Zhang,[2,3,*] and Hui Zhai[1,†]

[1]*Institute for Advanced Study, Tsinghua University, Beijing, 100084, China*
[2]*Institute for Quantum Information and Matter, California Institute of Technology, Pasadena, California 91125, USA*
[3]*Walter Burke Institute for Theoretical Physics, California Institute of Technology, Pasadena, California 91125, USA*

In this supplemental material, we present more details of magnetization learning, details of pattern recognition and, and details of gradient calculation.

## MAGNETIZATION LEARNING

In this section, we provide more details about magnetization learning. While we numerically generate the initial product state $|\phi\rangle$, first we randomly generate $N$ single-qubit states $|\varphi_i\rangle = \frac{1}{\sqrt{|a_i|^2+|b_i|^2}}(a_i|\uparrow\rangle + b_i|\downarrow\rangle)$, $(i = 1, 2\cdots N)$. To generate $a_i$ and $b_i$, we split them into real and imaginary part as $a_i = \frac{1}{\sqrt{2}}(a_i^{real} + ia_i^{imag})$, $b_i = \frac{1}{\sqrt{2}}(b_i^{real} + ib_i^{imag})$. Here $a_i^{real}, a_i^{imag}$ take the same normal distribution $\mathcal{N}(\mu, 0.2)$, and $b_i^{real}, b_i^{imag}$ take the distribution $\mathcal{N}(\text{sgn}(\mu)(1-|\mu|), 0.2)$. $\mu \in \{\pm 0.8, \pm 0.2\}$ is also randomly chosen. This procedure ensures a large initial magnetization. The product state is then given by $|\phi\rangle = \otimes_{i=1}^N |\varphi_i\rangle$

Because the Hamiltonian needed to be chaotic, the parameters of the Hamiltonian $J_\alpha^{ij}, h_\alpha^i$ in the main text take the normal distribution $\mathcal{N}(0, 2)$ and evolution time $t = 4\pi$. To make sure this unitary evolution is chaotic, we generate the unitary matrix to make sure the operator size $\text{Size}(\hat{\mathcal{U}}^\dagger \sum_{i=1}^N \hat{\sigma}_z^i \hat{\mathcal{U}})$ near $3N/4$.

The training and test dataset contain $N_D = 1000$ and 300 wavefunction-magnetization pairs. We use Adam algorithm to optimize the parameters of QNN. Momentum parameters are always $\beta_1 = 0.9$ and $\beta_2 = 0.999$. For different QNN structure, learning rates $\eta$ are same for $N_{unit} = 4, \eta = 0.01$ and $N_{unit} = 7, \eta = 0.005$. But the readout qubit is different. For (B), (C), ($\Lambda$), (H) and (S) quantum circuit structure, the readout qubits are $\hat{\sigma}_x^4, \hat{\sigma}_x^8, \hat{\sigma}_x^4, \hat{\sigma}_x^1, \hat{\sigma}_x^1$

## PATTERN RECOGNITION

In this section, we show some details of data generation from the "Street View of House Number" (SVHN) [1]. Here we use QNN to classify two classes, 6 and 9. Each image is $32 \times 32$ RGB image. Fig.[1] shows some examples of original training data set. In order to encode thes images to states in a 8-qubit system, first we resize these images to $16 \times 16$ pixels. Each pixel contains three channels $p_r, p_g, p_b \in \{0, 1, 2\cdots 255\}$. We encode these three integers to a complex number $c_k$, which is the coefficient of one basis $|\phi_k\rangle$ in the Hilbert space. $p_r^k, p_g^k, p_b^k$ are three eight-digit binary number of $k_{th}$ pixel. We join four-digit bits of three channels to $p_{real}^k$ and last four-digit bits to $p_{imag}^k$ shown in Fig.[2]. Then we convert them to decimal number $\tilde{p}_{real}^k, \tilde{p}_{imag}^k$ and $c_k = 1/2^{12}(\tilde{p}_{real}^k + i\tilde{p}_{imag}^k)$. Consequently, each image is encoded to a wavefunction $|\psi\rangle = \sum_{k=1}^{256} c_k|\phi_k\rangle/Z$ and $|\phi_k\rangle$ is the computational basis of this 8-qubit system's Hilbert space, $Z^2 = 1/\sum_{k=1}^{256}|c_k|^2$ is the normalization of $|\psi\rangle$. The label of "6" is 0 and "9" is 1. The training and test dataset also contains $N_D = 1000$ and 300 images with equal number of data within the two classes.

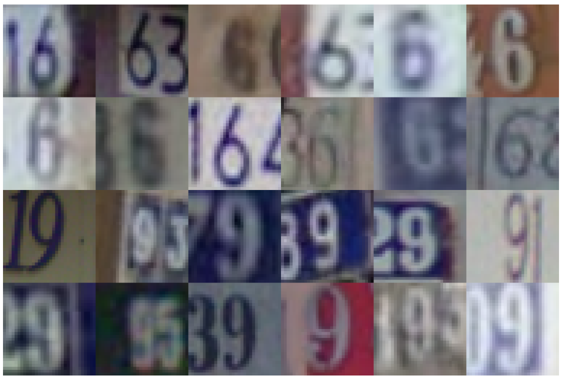

FIG. 1: Original RGB images of SVHN data set. First two rows are in the class "6" and last two rows are in the class "9".

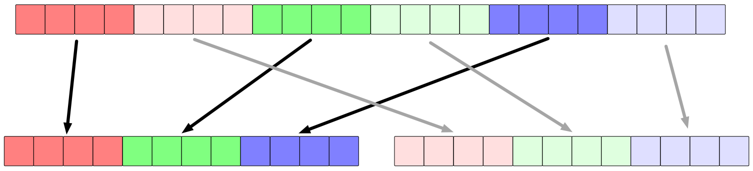


FIG. 2: Encoding three channels of each pixel to a complex number. Each grid is a binary number and after joint, we convert these two 12-digit binary number to decimal number.

## GRADIENTS IN QUANTUM NEURAL NETWORKS

In this section, we show the method of computing the gradients of quantum neural networks in this work. For a quantum circuit contains $L$ layers, $\hat{\mathcal{U}} = \hat{U}_1\hat{U}_2\cdots\hat{U}_L = \prod_{l=1}^{L}\hat{U}_l$. For the $l$ layer $\hat{U}_l$ it contains $N_l$ two-qubit gates. Each two-qubit gate is a $4\times 4$ matrix in the SU(4) group and can be parameterized by 15 parameters.

$$\hat{\mathcal{U}} = \hat{U}_1\hat{U}_2\cdots\hat{U}_L = \prod_{l=1}^{L}\hat{U}_l \tag{1}$$

$$\hat{U}_l = \hat{U}_{l1}\otimes\cdots\otimes\hat{U}_{lN_l} = \otimes_{n_l=1}^{N_l}\hat{U}_{ln_l} \tag{2}$$

$$\hat{U}_{ln_l} = \exp(\sum_{k=1}^{15} a_{ln_l}^k \hat{g}_k) \tag{3}$$

All of the SU(4) group parameters $\{a_{ln_l}^k\}$ should be optimized.

Generally, a loss function of a QNN is a function of this unitary $\mathcal{L} = \mathcal{L}(\hat{\mathcal{U}})$. The gradient of these parameters are:

$$\frac{\partial\mathcal{L}}{\partial a_{ln_l}^k} = \frac{\partial\mathcal{L}}{\partial\hat{\mathcal{U}}}\frac{\partial\hat{\mathcal{U}}}{\partial a_{ln_l}^k} \tag{4}$$

$$\frac{\partial\hat{\mathcal{U}}}{\partial a_{ln_l}^k} = \hat{U}_1\cdots\frac{\partial\hat{U}_l}{\partial a_{ln_l}^k}\cdots\hat{U}_L \tag{5}$$

$$\frac{\partial\hat{U}_l}{\partial a_{ln_l}^k} = \hat{U}_{l1}\otimes\cdots\otimes\frac{\partial\hat{U}_{ln_l}}{\partial a_{ln_l}^k}\otimes\cdots\otimes\hat{U}_{lN_l} \tag{6}$$

The key is the gradient of this exponential matrix $\frac{\partial\hat{U}_{ln_l}}{\partial a_{ln_l}^k}$

*Matrix Exponential Gradient.* Generally a matrix exponential gradient [2] is

$$\frac{d}{dt}e^{\hat{X}(t)} = \int_0^1 e^{s\hat{X}(t)}\frac{d\hat{X}(t)}{dt}e^{(1-s)\hat{X}(t)}ds. \tag{7}$$

We consider the case with $\hat{X}(t) = \hat{A} + \hat{B}t$:

$$\frac{d}{dt}e^{\hat{A}+\hat{B}t}|_{t=0} = \left[\int_0^1 e^{\hat{A}s}\hat{B}e^{-\hat{A}s}ds\right]e^{\hat{A}}. \tag{8}$$

We define

$$\hat{M}(t) = e^{-\hat{A}t}\int_0^t e^{\hat{A}s}\hat{B}e^{-\hat{A}s}ds, \qquad \hat{N}(t) = e^{\hat{A}t}. \tag{9}$$

This leads to

$$\frac{d}{dt}e^{\hat{A}+\hat{B}t}|_{t=0} = e^{\hat{A}}\hat{M}(1)e^{\hat{A}}. \tag{10}$$

Taking the time gradient of eq.(9) gives

$$\frac{d}{dt}\begin{pmatrix}\hat{M}(t)\\ \hat{N}(t)\end{pmatrix}=\begin{pmatrix}-\hat{A} & \hat{B}\\ \hat{0} & -\hat{A}\end{pmatrix}\begin{pmatrix}\hat{M}(t)\\ \hat{N}(t)\end{pmatrix}. \tag{11}$$

With the initial condition $\hat{M}(0)=\hat{0}, \hat{N}=\hat{1}$, we can obtain $\hat{M}(1)$. To apply this method to the gradient of the parameters in the QNN, we consider

$$\hat{A}=\sum_{j=1}^{15} a^{j}_{l n_l}\hat{g}_j, \qquad \hat{B}=\hat{g}_k. \tag{12}$$

$\frac{\partial \hat{U}_{l n_l}}{\partial a^{k}_{l n_l}}$ is then given by (10).

* Electronic address: pengfeizhang.physics@gmail.com
† Electronic address: hzhai@tsinghua.edu.cn
[1] Yuval Netzer, Tao Wang, Adam Coates, Alessandro Bissacco, Bo Wu, and Andrew Y. Ng, "Reading Digits in Natural Images with Unsupervised Feature Learning," NIPS Workshop on Deep Learning and Unsupervised Feature Learning (2011).
[2] Cleve Moler, and Charles Van Loan, "Nineteen dubious ways to compute the exponential of a matrix, twenty-five years later," SIAM Rev. **45**(**1**),3 – 49 (2003).
